# Supplementary material for: High-temperature multigap superconductivity in two-dimensional metal-borides
Source: arXiv:2112.04317 source file (2021-12-08)
Supplement: Supplementary file 1 [file Supplementary_materials.pdf]

# High-temperature multigap superconductivity in two-dimensional metal-borides

Cem Sevik[1, 2], Mikhail Petrov[1], Jonas Bekaert[1], and Milorad V. Milosevic[1],
[1]Department of Physics & NANOlab Center of Excellence, University of Antwerp, Groenenborgerlaan 171, B-2020 Antwerp, Belgium
[2]Department of Mechanical Engineering, Faculty of Engineering, Eskisehir Technical University, 26555 Eskisehir, Turkey

## Structures

| $M_2B_2$ | $MB_4$ | $MB_2$ |
|---|---|---|
| 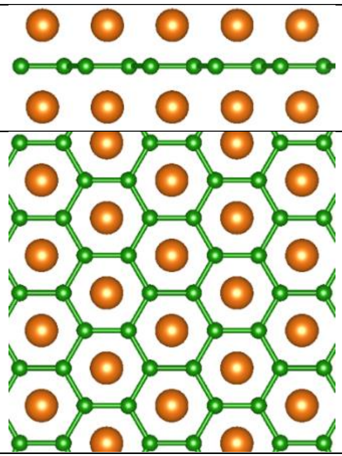 | 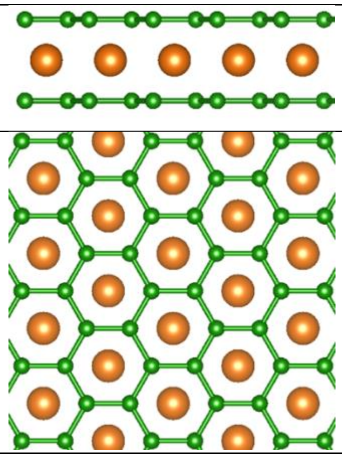 | 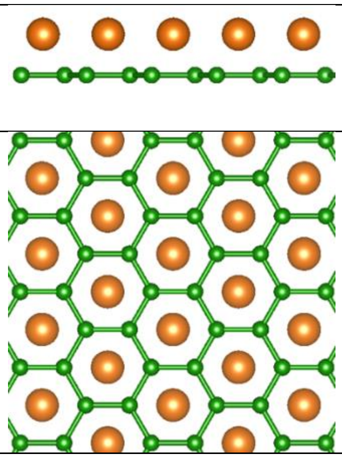 |

## Cohesive Energies (in eV)

| Metal | $MB_4$ | $MB_2$ | $M_2B_2$ | Metal | $MB_4$ | $MB_2$ | $M_2B_2$ |
|---|---|---|---|---|---|---|---|
| Be | 5.32 | 5.15 | 4.51 | V | 6.04 | 5.58 | 5.76 |
| Mg | 4.86 | 4.20 | 3.75 | Nb | 6.40 | 6.14 | 6.68 |
| Ca | 4.83 | 4.17 | 4.00 | Ta | 6.64 | 6.48 | 7.16 |
| Sc | 5.70 | 5.33 | 5.56 | Cr | 5.60 | 4.94 | 4.75 |
| Ti | 6.38 | 6.22 | 6.77 | Mo | 6.15 | 5.73 | 5.95 |
| Zr | 6.38 | 6.29 | 7.04 | W | 6.55 | 6.35 | 6.75 |
| Hf | 6.41 | 6.28 | 6.99 | Re | 6.27 | 6.10 | 6.30 |
| Al | 5.27 | 4.73 | 4.42 | | | | |

## Lattice Constants

| Materials | $a_0$ (Å) | Materials | $a_0$ (Å) | Materials | $a_0$ (Å) |
|---|---|---|---|---|---|
| $BeB_4$ | 2.968 | $ZrB_4$ | 3.119 | $CrB_4$ | 2.910 |
| $MgB_4$ | 3.007 | $HfB_4$ | 3.109 | $MoB_4$ | 2.966 |
| $CaB_4$ | 3.075 | $VB_4$ | 2.959 | $WB_4$ | 2.966 |
| $ScB_4$ | 3.080 | $NbB_4$ | 3.045 | $ReB_4$ | 2.929 |
| $TiB_4$ | 3.028 | $TaB_4$ | 3.045 | $AlB_4$ | 2.991 |

| Materials | $a_0$ (Å) | Materials | $a_0$ (Å) | Materials | $a_0$ (Å) |
|---|---|---|---|---|---|
| $BeB_2$ | 3.050 | $ZrB_2$ | 3.152 | $CrB_2$ | 3.128 |
| $MgB_2$ | 3.044 | $HfB_2$ | 3.149 | $MoB_2$ | 2.918 |
| $CaB_2$ | 3.220 | $VB_2$ | 3.064 | $WB_2$ | 2.900 |
| $ScB_2$ | 3.176 | $NbB_2$ | 2.997 | $ReB_2$ | 2.882 |
| $TiB_2$ | 3.106 | $TaB_2$ | 3.002 | $AlB_2$ | 2.981 |

| Materials | $a_0$ (Å) | Materials | $a_0$ (Å) | Materials | $a_0$ (Å) |
|---|---|---|---|---|---|
| **$Be_2B_2$** | 2.905 | **$Zr_2B_2$** | 3.172 | **$Cr_2B_2$** | 2.932 |
| **$Mg_2B_2$** | 3.104 | **$Hf_2B_2$** | 3.129 | **$Mo_2B_2$** | 3.065 |
| **$Ca_2B_2$** | 3.364 | **$V_2B_2$** | 2.962 | **$W_2B_2$** | 3.039 |
| **$Sc_2B_2$** | 3.148 | **$Nb_2B_2$** | 3.110 | **$Re_2B_2$** | 2.916 |
| **$Ti_2B_2$** | 3.014 | **$Ta_2B_2$** | 3.075 | **$Al_2B_2$** | 2.943 |

**Critical Temperatures**

| Materials | Tc (K) | Materials | Tc (K) | Materials | Tc (K) |
|---|---|---|---|---|---|
| **$BeB_4$** | 29.9 | **$ZrB_4$** | Unstable | **$CrB_4$** | 0.0 |
| **$MgB_4$** | 22.2 | **$HfB_4$** | Unstable | **$MoB_4$** | 0.0 |
| **$CaB_4$** | 36.1 | **$VB_4$** | Unstable | **$WB_4$** | 0.0 |
| **$ScB_4$** | 10.4 | **$NbB_4$** | 0.0 | **$ReB_4$** | Unstable |
| **$TiB_4$** | Unstable | **$TaB_4$** | 0.0 | **$AlB_4$** | 30.9 |

| Materials | Tc (K) | Materials | Tc (K) | Materials | Tc (K) |
|---|---|---|---|---|---|
| **$BeB_2$** | 0.0 | **$ZrB_2$** | 2.9 | **$CrB_2$** | 4.5 |
| **$MgB_2$** | 11.6 | **$HfB_2$** | 0.8 | **$MoB_2$** | 0.2 |
| **$CaB_2$** | 41.6 | **$VB_2$** | 8.3 | **$WB_2$** | 0.0 |
| **$ScB_2$** | 20.4 | **$NbB_2$** | 35.5 | **$ReB_2$** | 2.4 |
| **$TiB_2$** | 0.0 | **$TaB_2$** | 7.1 | **$AlB_2$** | 9.8 |

| Materials | Tc (K) | Materials | Tc (K) | Materials | Tc (K) |
|---|---|---|---|---|---|
| **$Be_2B_2$** | Unstable | **$Zr_2B_2$** | 0.0 | **$Cr_2B_2$** | 0.5 |
| **$Mg_2B_2$** | 3.2 | **$Hf_2B_2$** | 0.0 | **$Mo_2B_2$** | 0.4 |
| **$Ca_2B_2$** | 1.3 | **$V_2B_2$** | 0.0 | **$W_2B_2$** | 0.3 |
| **$Sc_2B_2$** | 0.0 | **$Nb_2B_2$** | 0.0 | **$Re_2B_2$** | 5.5 |
| **$Ti_2B_2$** | 0.0 | **$Ta_2B_2$** | 0.0 | **$Al_2B_2$** | 0.0 |

**The Calculated Phonon Dispersion, Electronic Band Structures, $\alpha^2F$, and $\lambda$**

The calculated phonon dispersion / atom resolved phonon density of states (left), electronic band structure (Right Top), and $\alpha^2F$ (blue solid line) / $\lambda$ (red dashed line) (right bottom) for all the considered materials are presented below. The red and green dashed lines in atom resolved phonon density of states represent the contribution of Metal and Boron atoms, respectively.

**$M_2B_2$ Crystals**

$Be_2B_2$ UNSTABLE

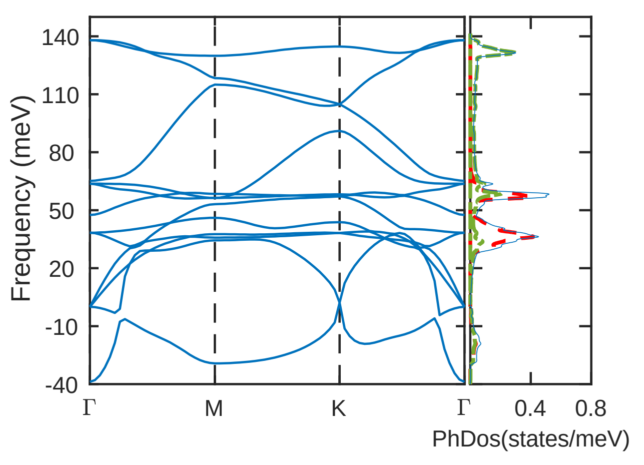


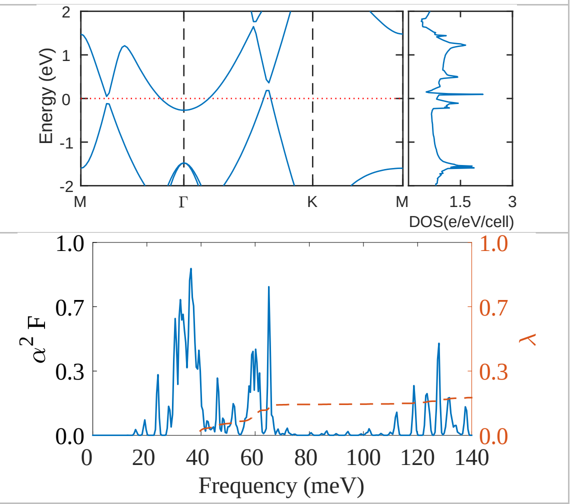

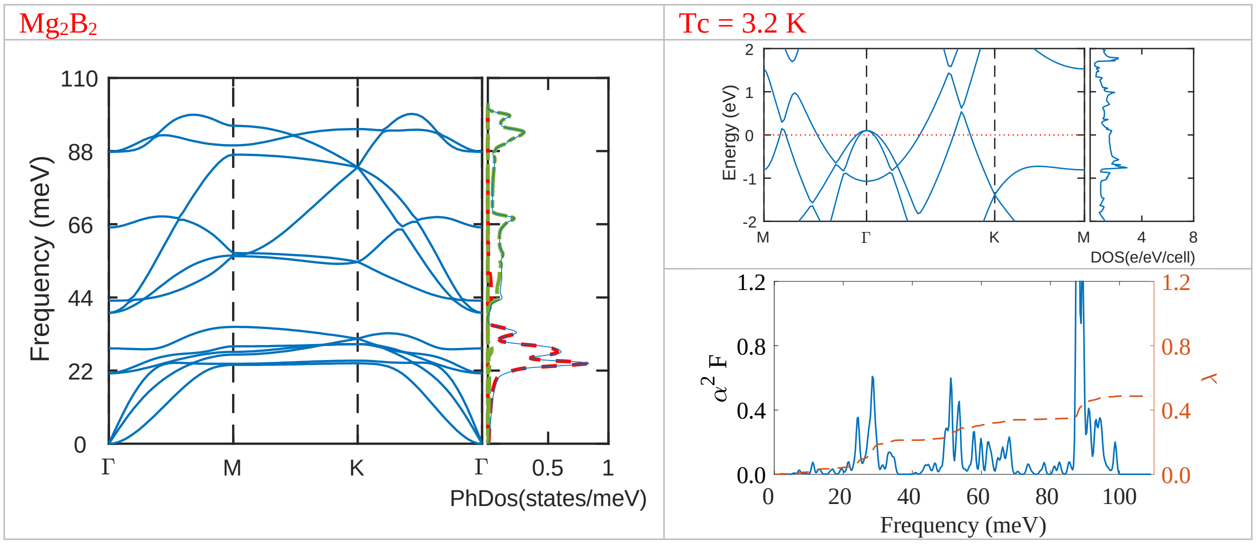
Mg2B2
Tc = 3.2 K
Frequency (meV)
Γ M K Γ
PhDos(states/meV)
Energy (eV)
DOS(e/eV/cell)
α2 F
λ
Frequency (meV)

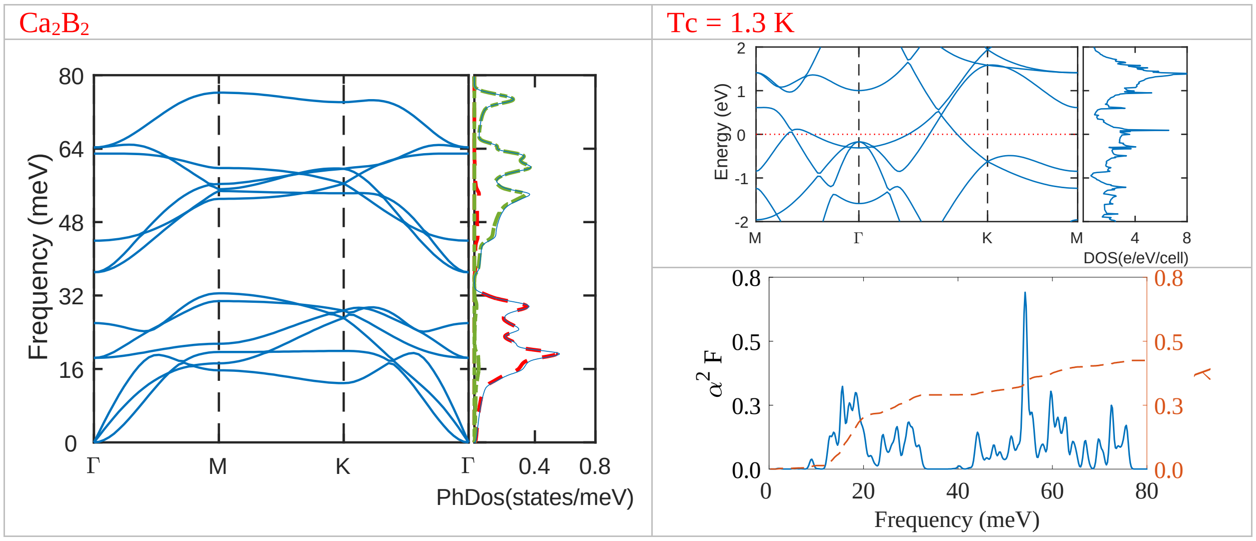
Ca2B2
Tc = 1.3 K
Frequency (meV)
Γ M K Γ
PhDos(states/meV)
Energy (eV)
DOS(e/eV/cell)
α2 F
λ
Frequency (meV)

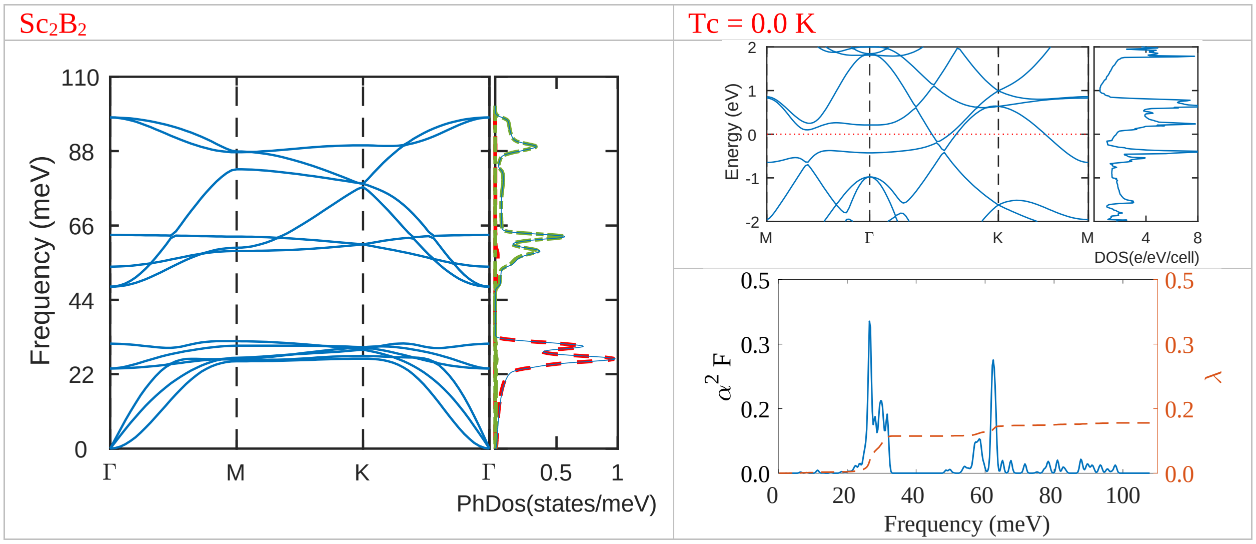
Sc2B2
Tc = 0.0 K
Frequency (meV)
Γ M K Γ
PhDos(states/meV)
Energy (eV)
DOS(e/eV/cell)
α2 F
λ
Frequency (meV)

| $Ti_2B_2$ | Tc = 0.0 K |
|---|---|

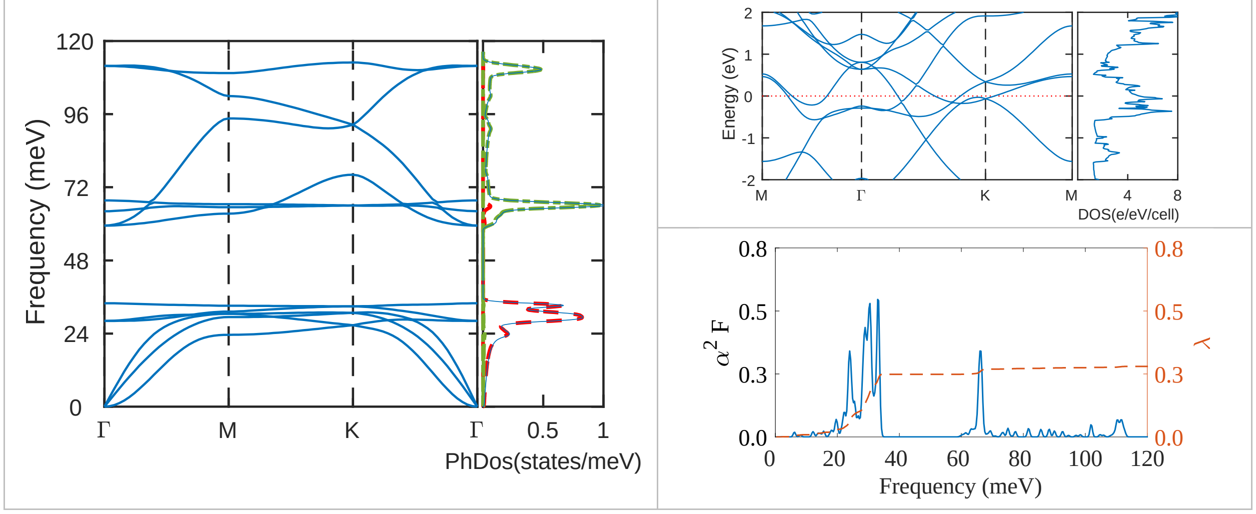


| $Zr_2B_2$ | Tc = 0.0 K |
|---|---|

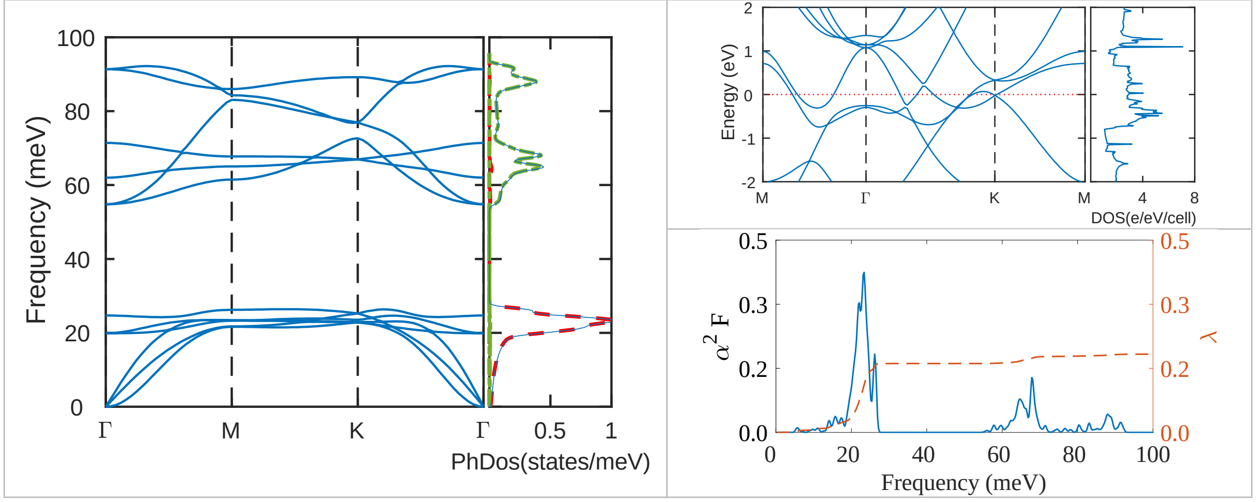


| $Hf_2B_2$ | Tc = 0.0 K |
|---|---|

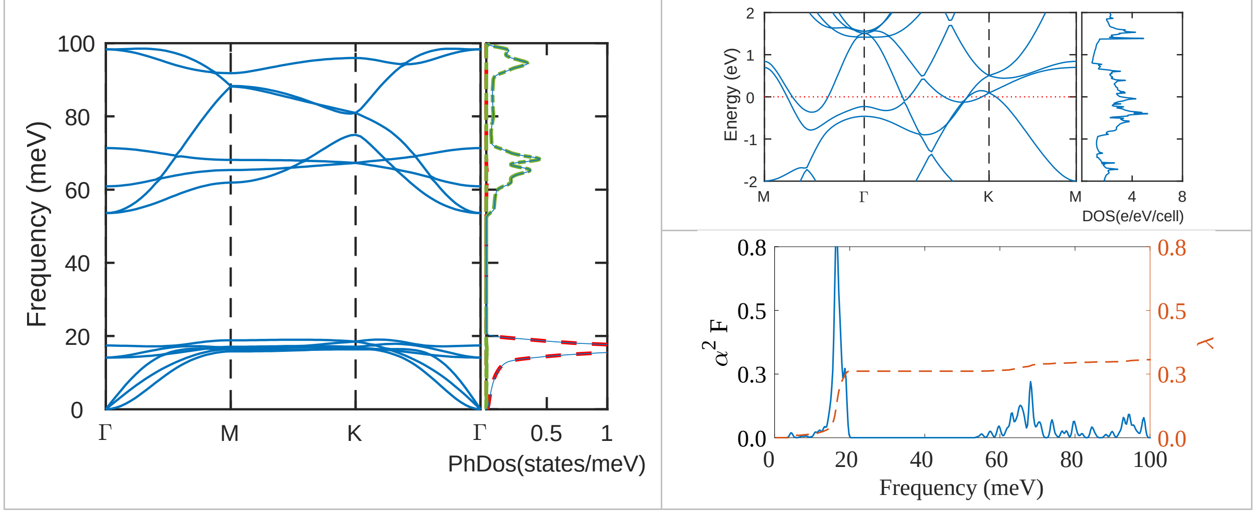

$V_2B_2$ — Tc = 0.0 K

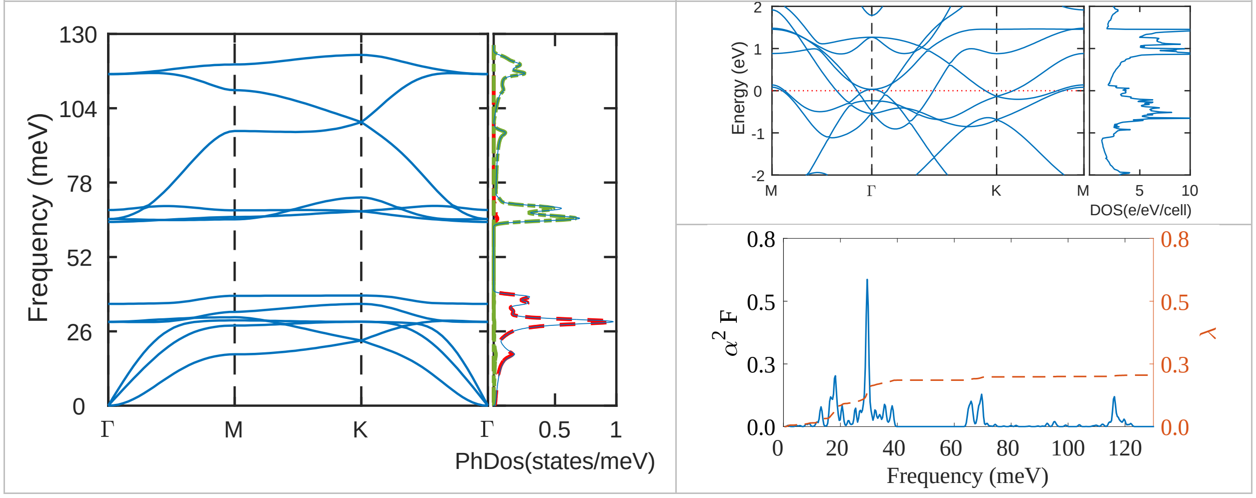


$Nb_2B_2$ — Tc = 0.0 K

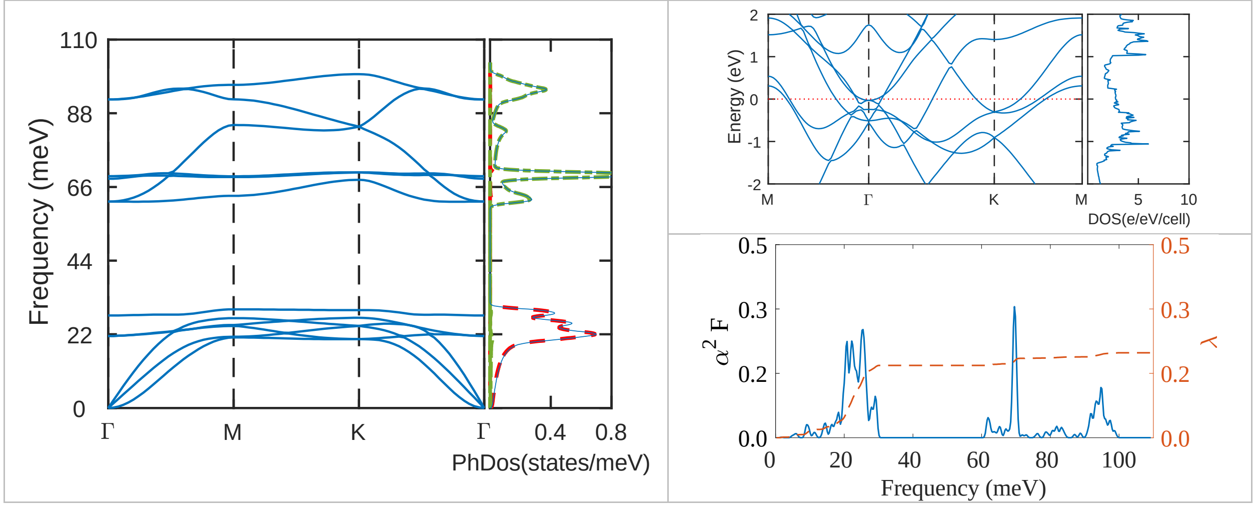


$Ta_2B_2$ — Tc = 0.0 K

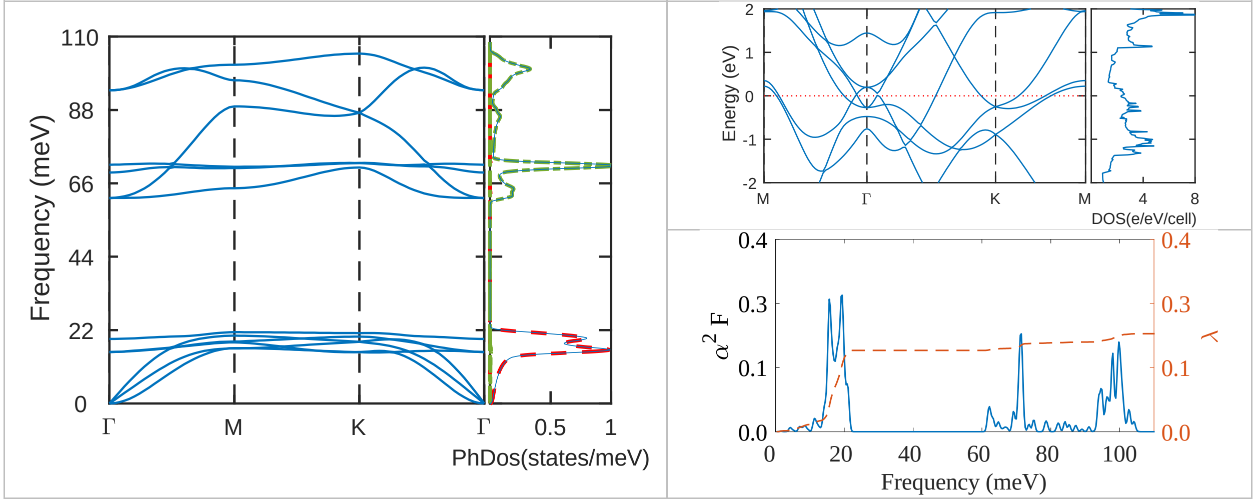

$Cr_2B_2$ Tc = 0.5 K

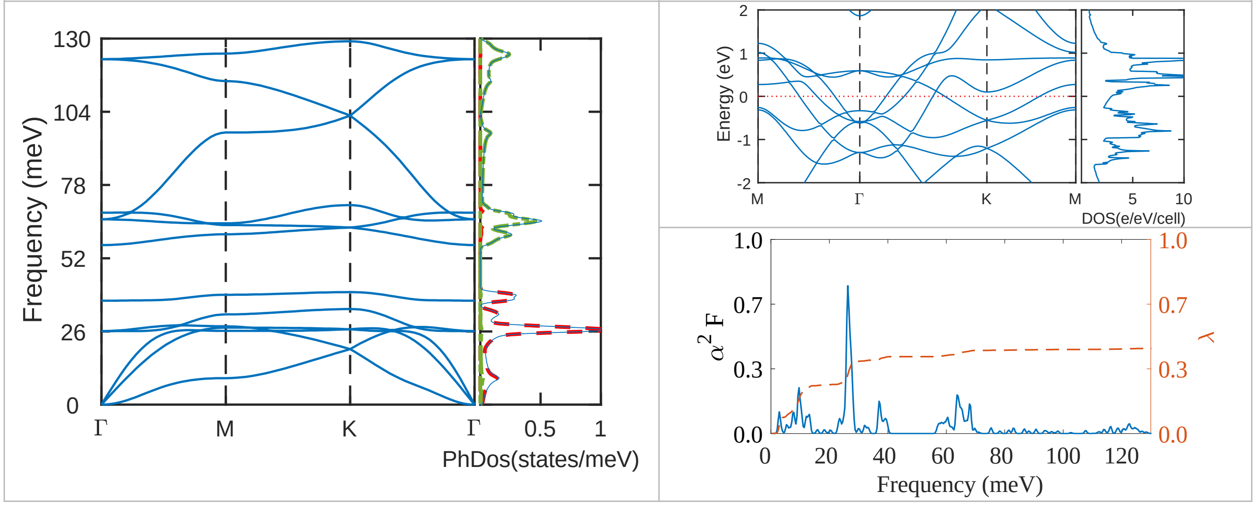


$Mo_2B_2$ Tc = 0.4 K

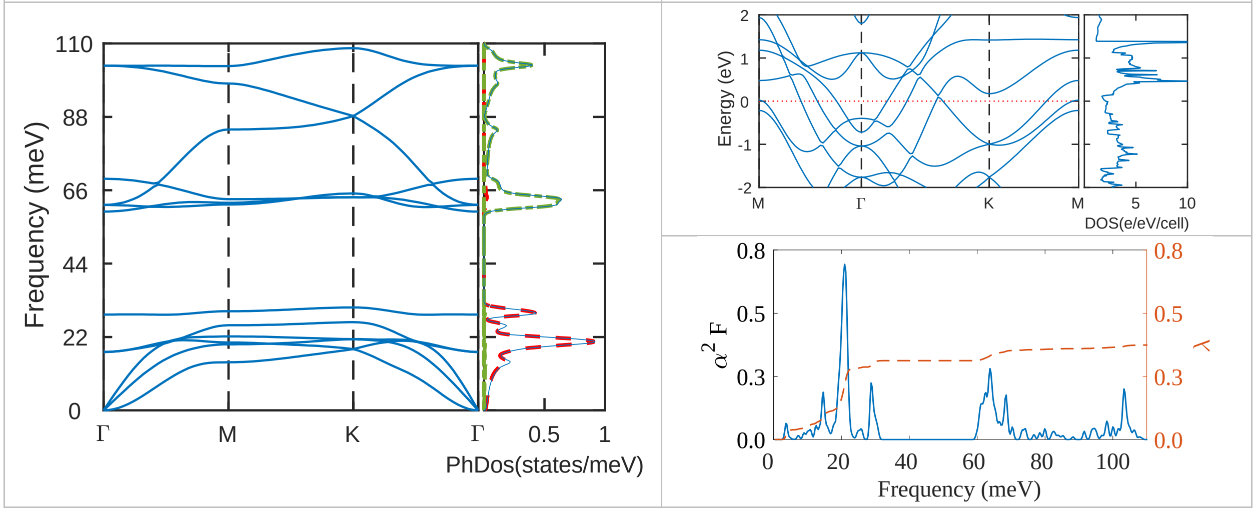


$W_2B_2$ Tc = 0.3 K

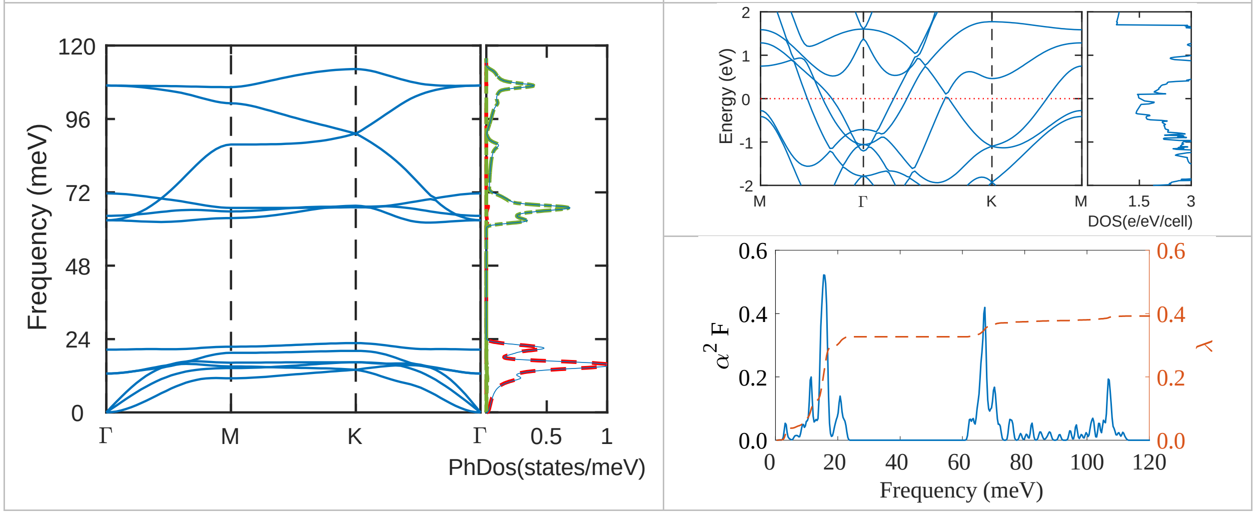

$Re_2B_2$ | Tc = 5.5 K

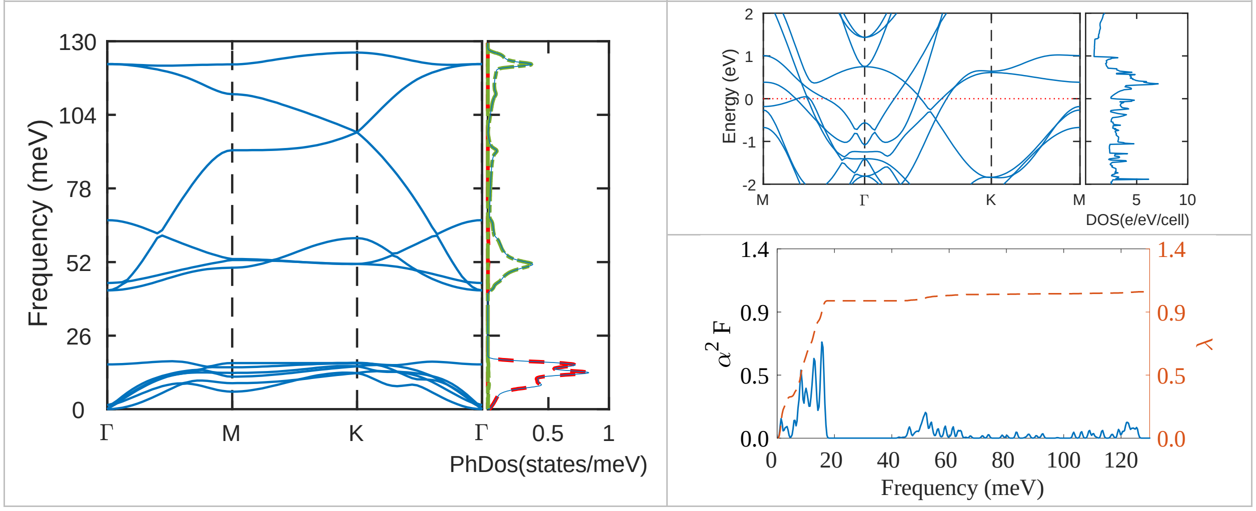


$Al_2B_2$ | Tc = 0.0 K

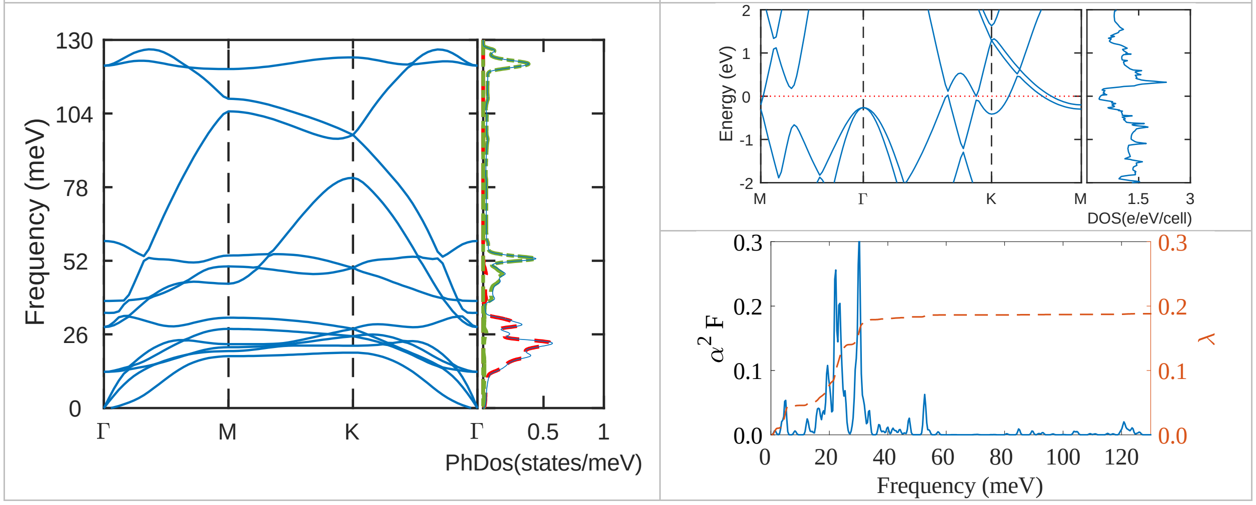


**$MB_4$ Crytals**

$BeB_4$ | Tc = 29.9 K

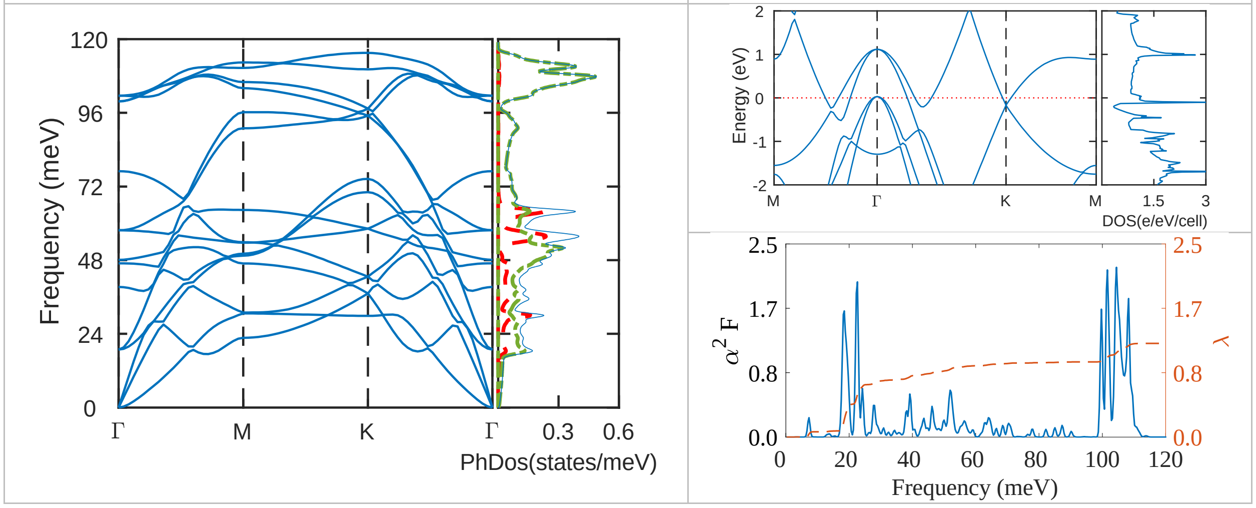

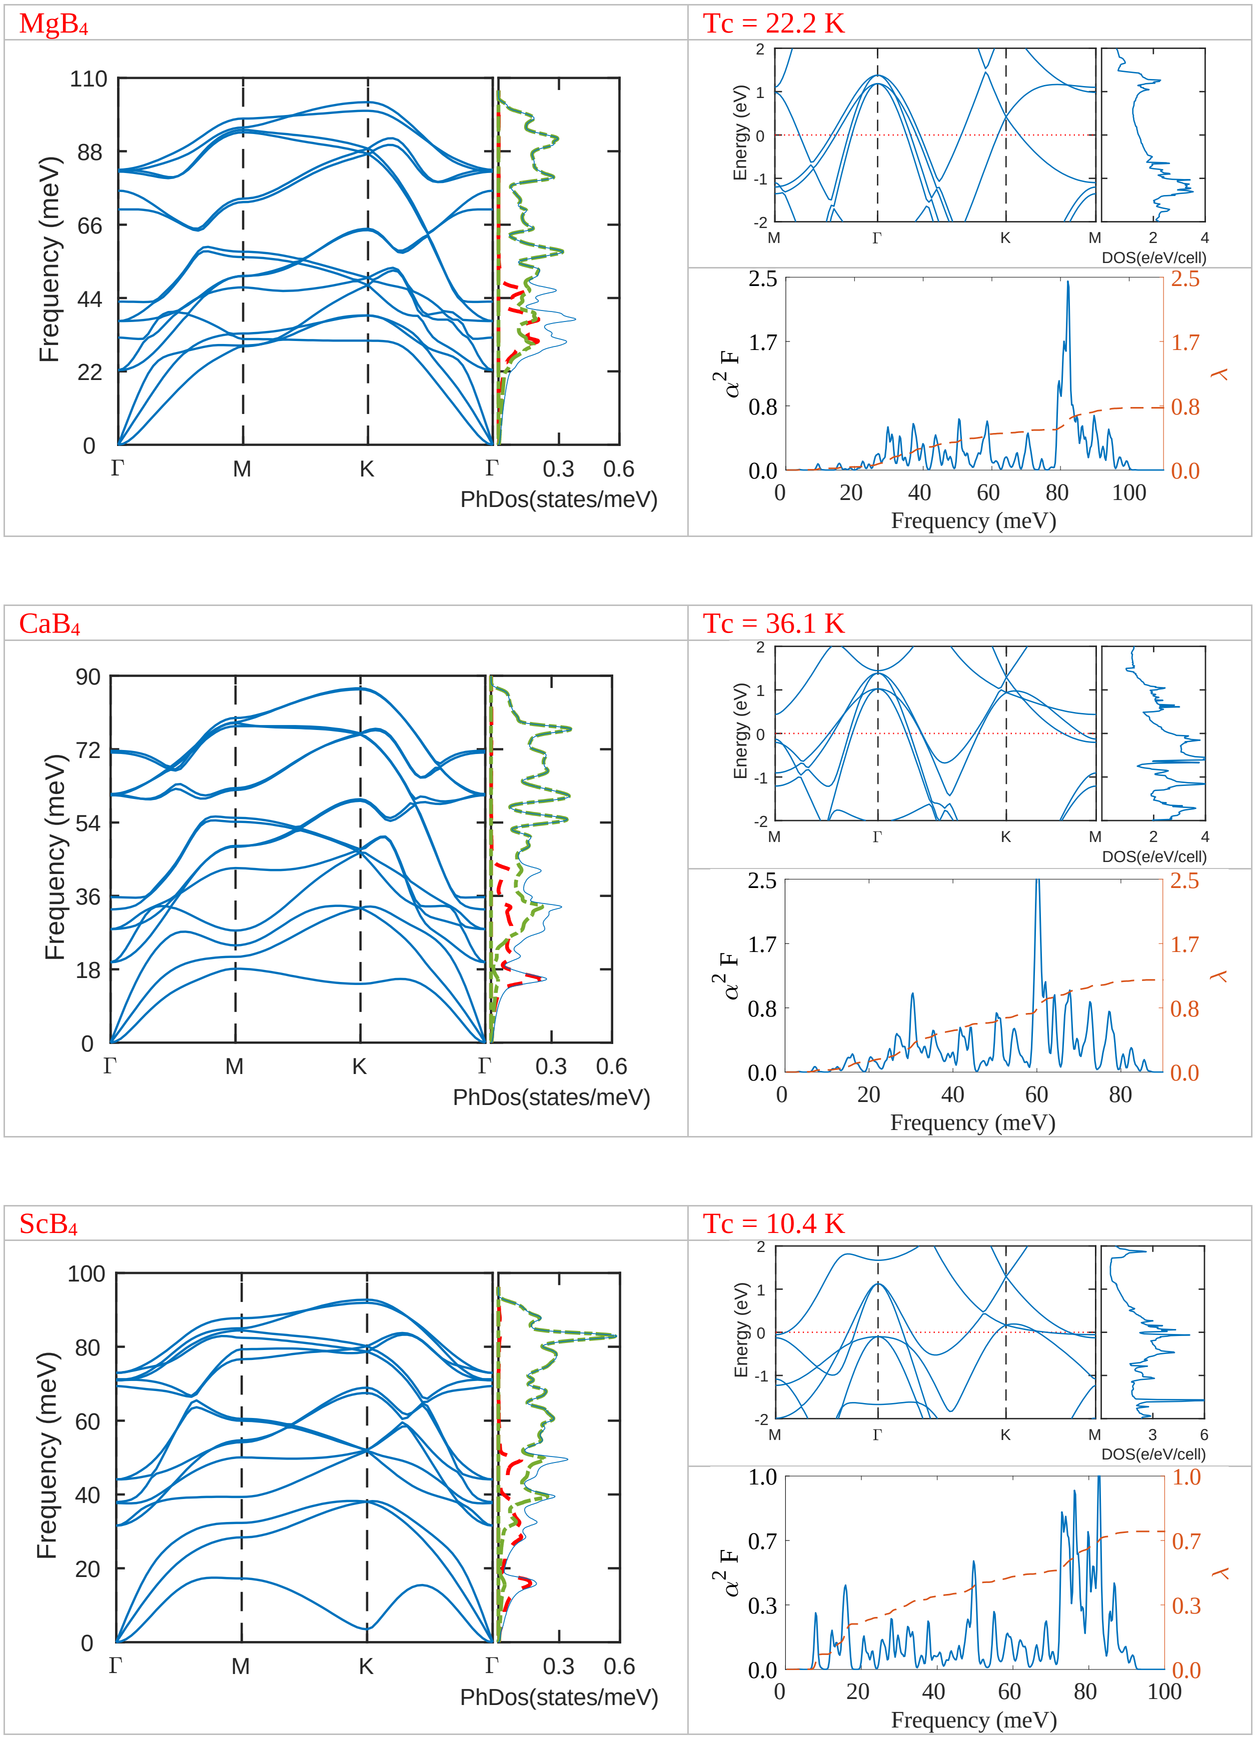

MgB4
Tc = 22.2 K
Frequency (meV)
Γ
M
K
PhDos(states/meV)
Energy (eV)
DOS(e/eV/cell)
α2 F
λ
CaB4
Tc = 36.1 K
ScB4
Tc = 10.4 K

$TiB_4$

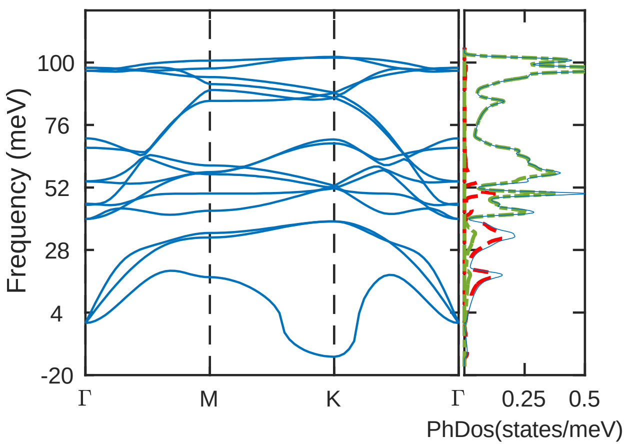


Tc = /

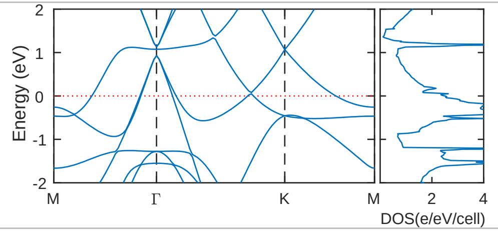


UNSTABLE

$ZrB_4$

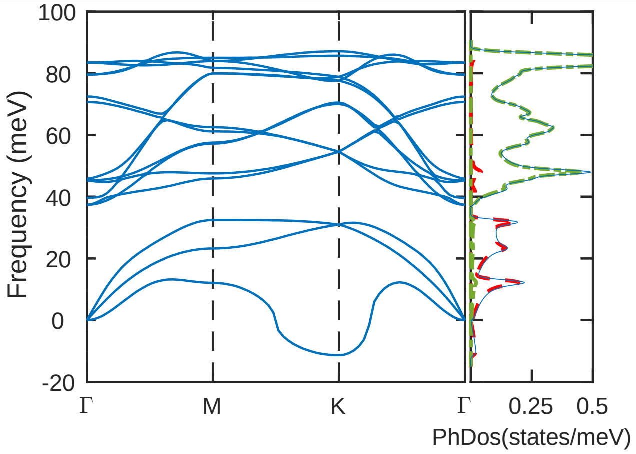


Tc = /

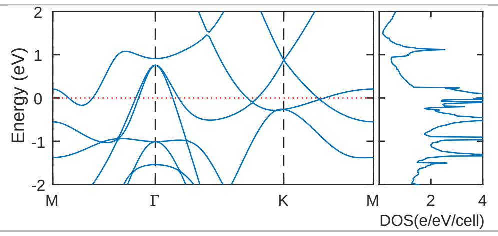


UNSTABLE

$HfB_4$

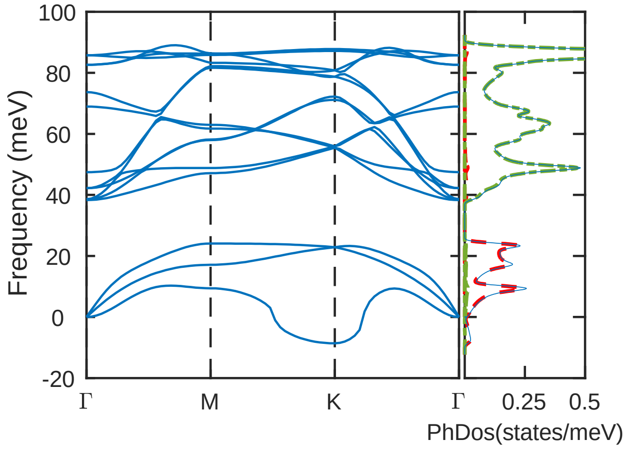


Tc = /

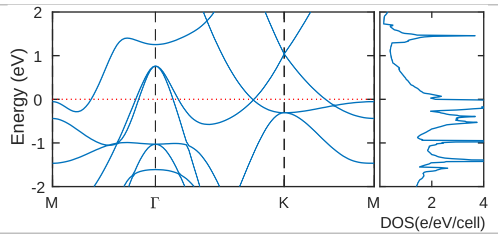


UNSTABLE

| $VB_4$ | Tc = 0.0 K |
|---|---|

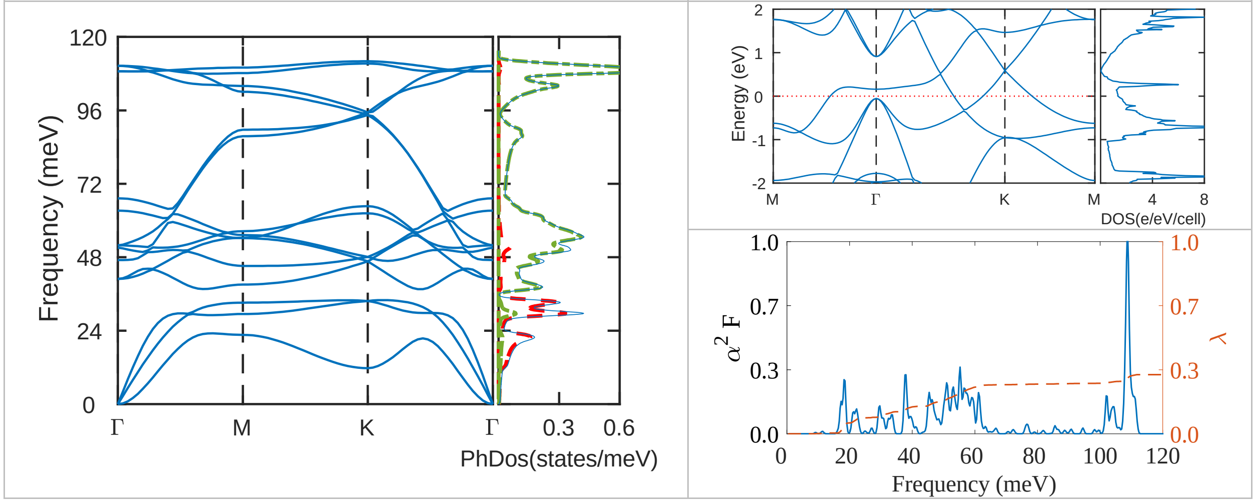


| $NbB_4$ | Tc = 0.0 K |
|---|---|

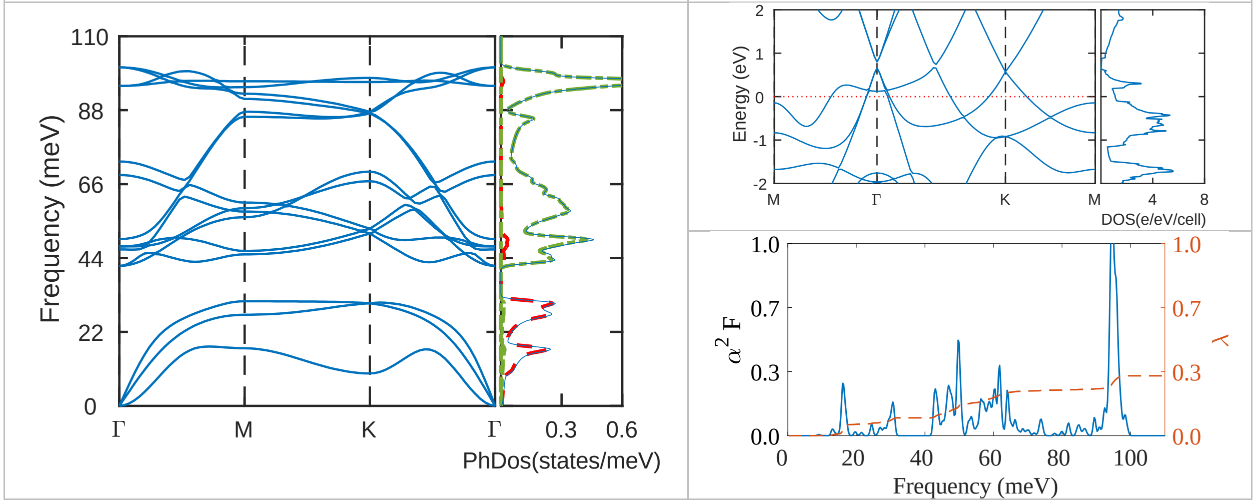


| $TaB_4$ | Tc = 0.0 K |
|---|---|

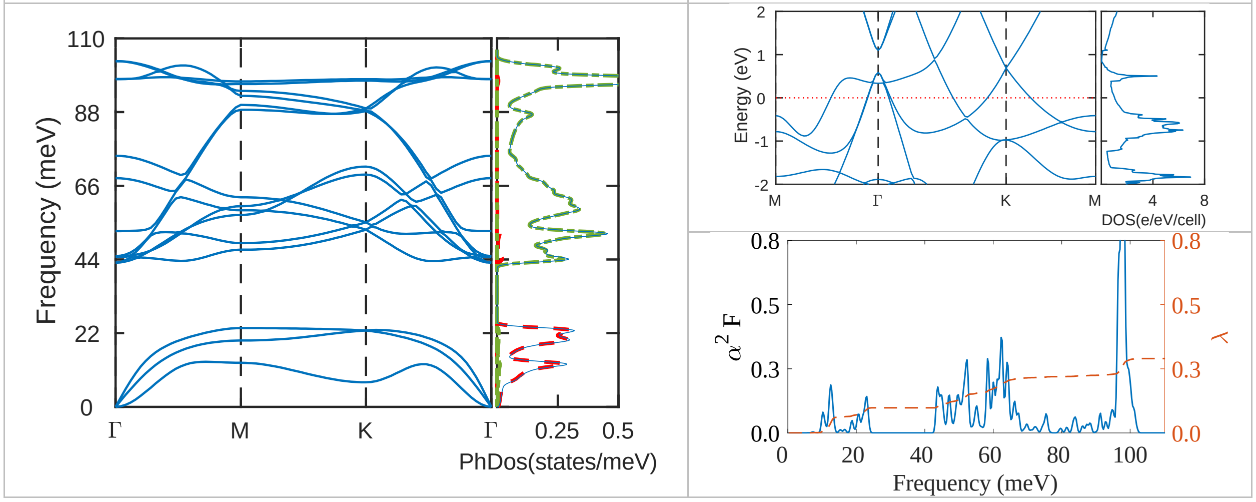

| $CrB_4$ | Tc = 0.0 |
|---|---|

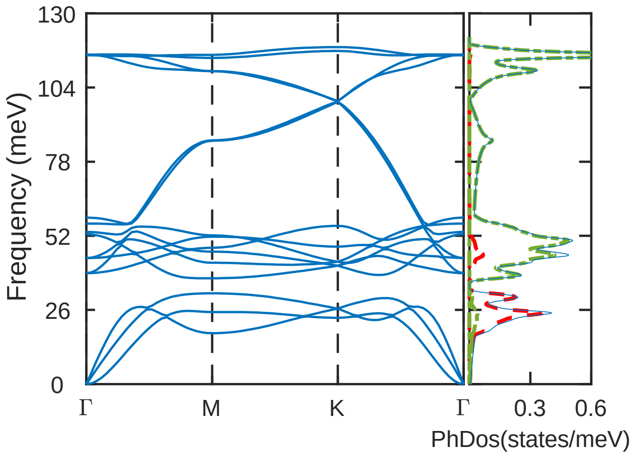


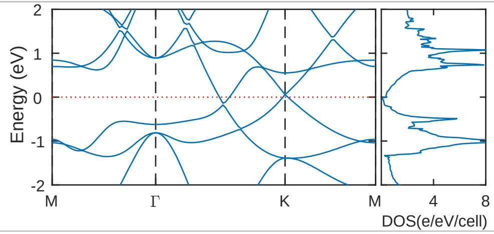


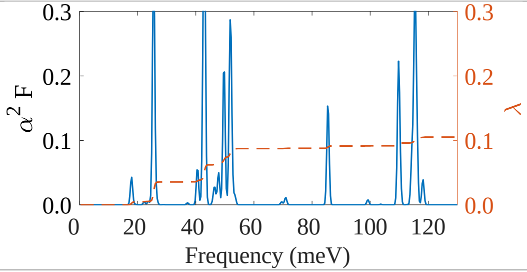


| $MoB_4$ | Tc = 0.0 K |
|---|---|

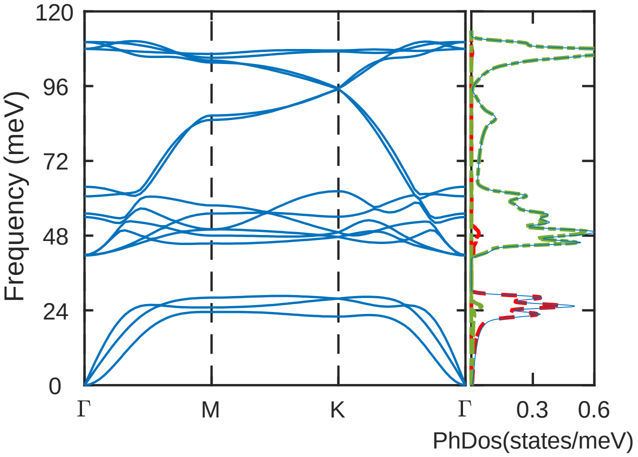


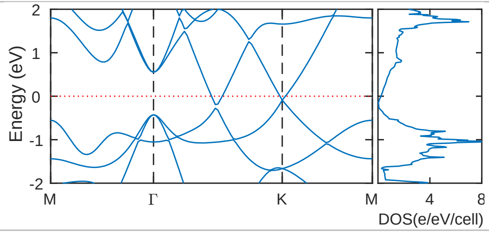


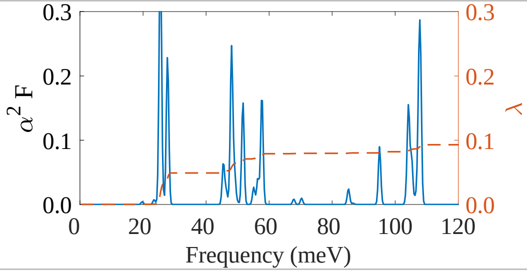


| $WB_4$ | Tc = 0.0 K |
|---|---|

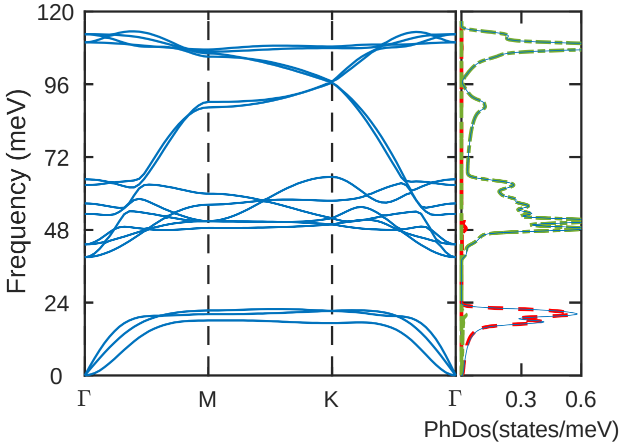


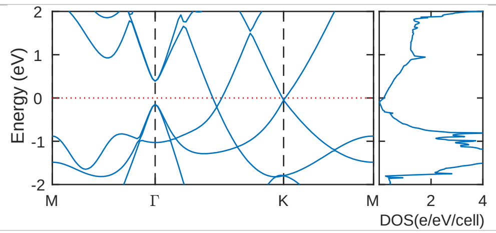


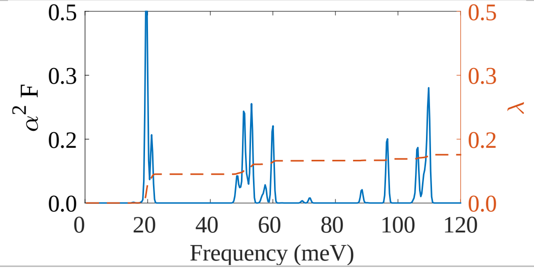

$ReB_4$ | Tc = /

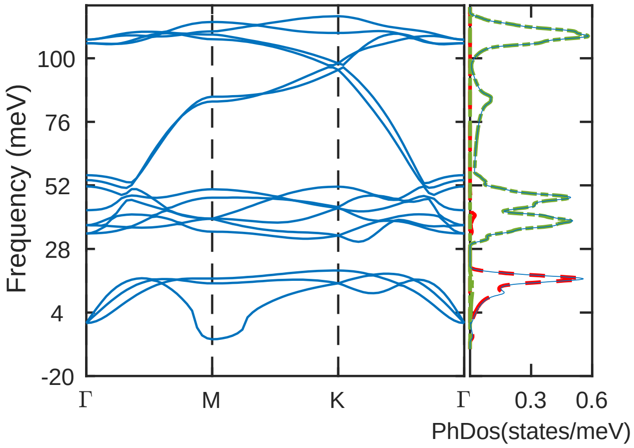


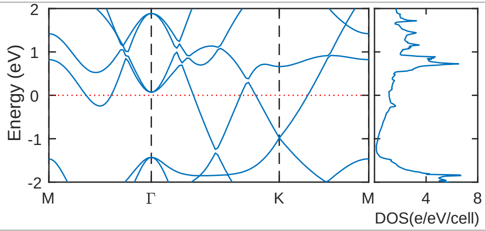


UNSTABLE

$AlB_4$ | Tc = 30.9 K

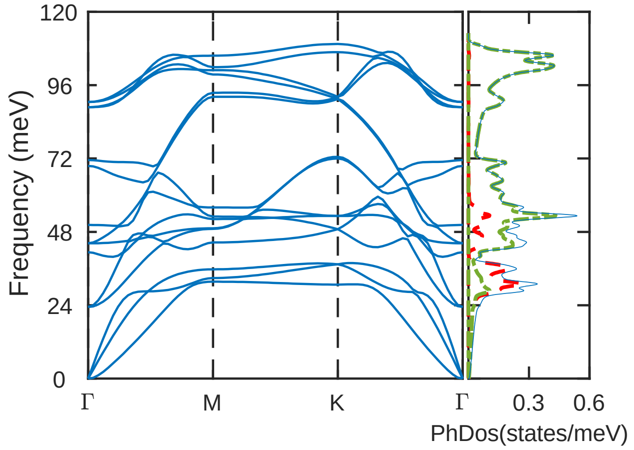


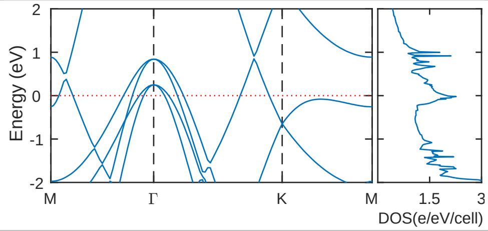


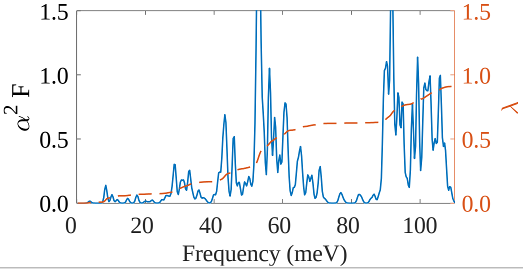


**$MB_2$ Crystals**

$BeB_2$ | Tc = 0.0 K

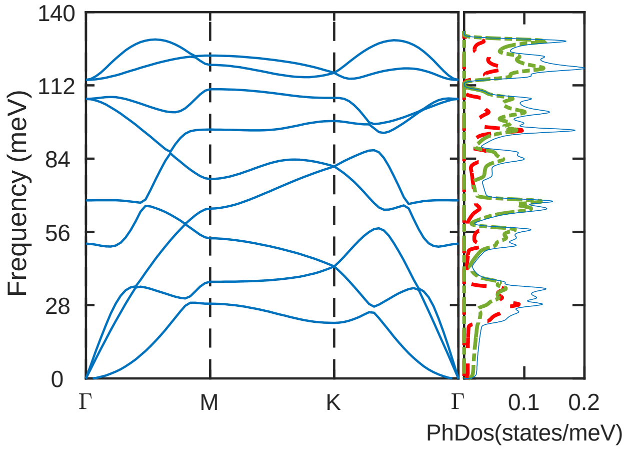


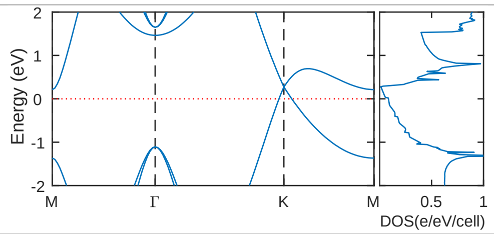


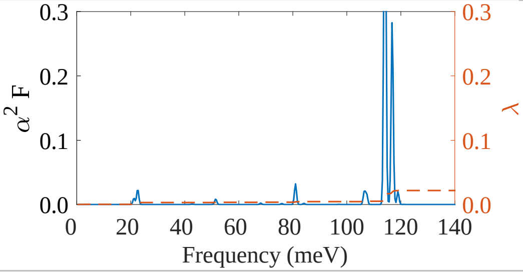

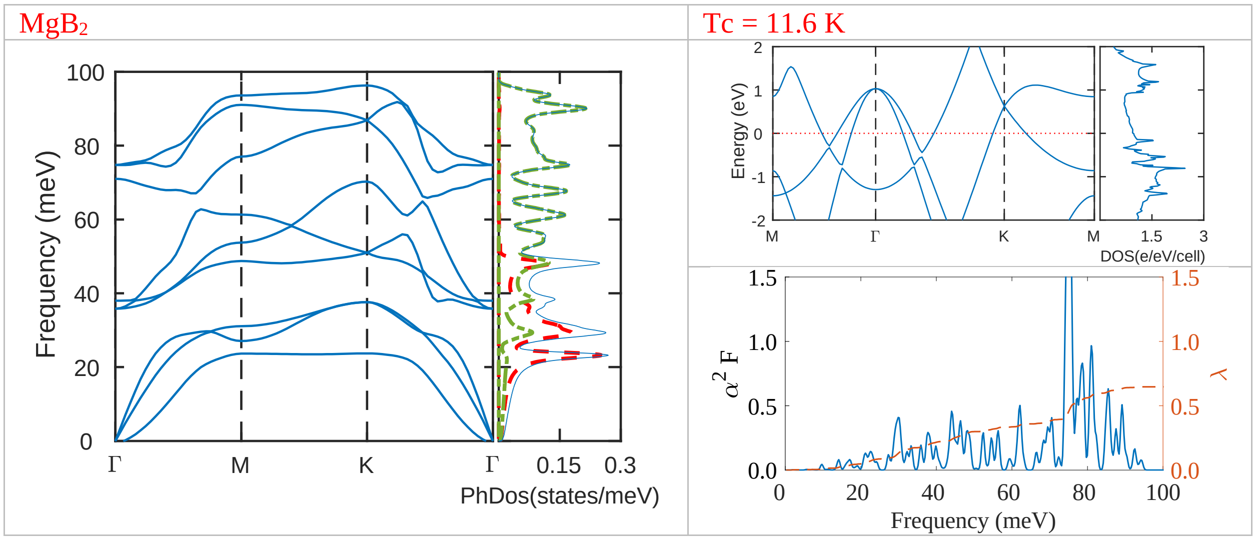
MgB₂
Tc = 11.6 K
Frequency (meV)
PhDos(states/meV)
Energy (eV)
DOS(e/eV/cell)
α² F
λ
Frequency (meV)

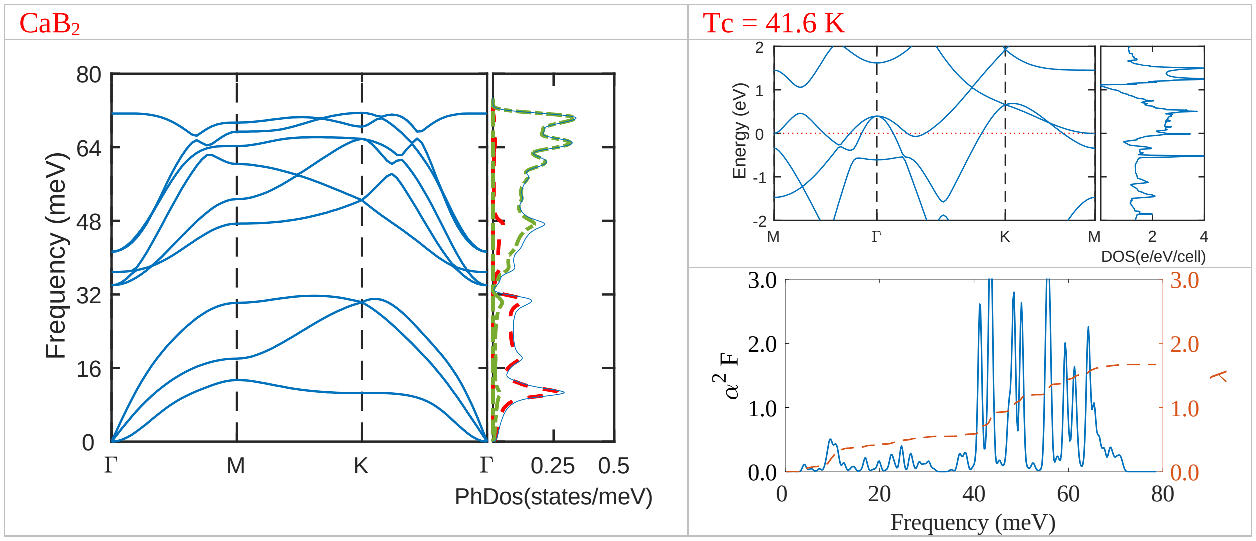
CaB₂
Tc = 41.6 K
Frequency (meV)
PhDos(states/meV)
Energy (eV)
DOS(e/eV/cell)
α² F
λ
Frequency (meV)

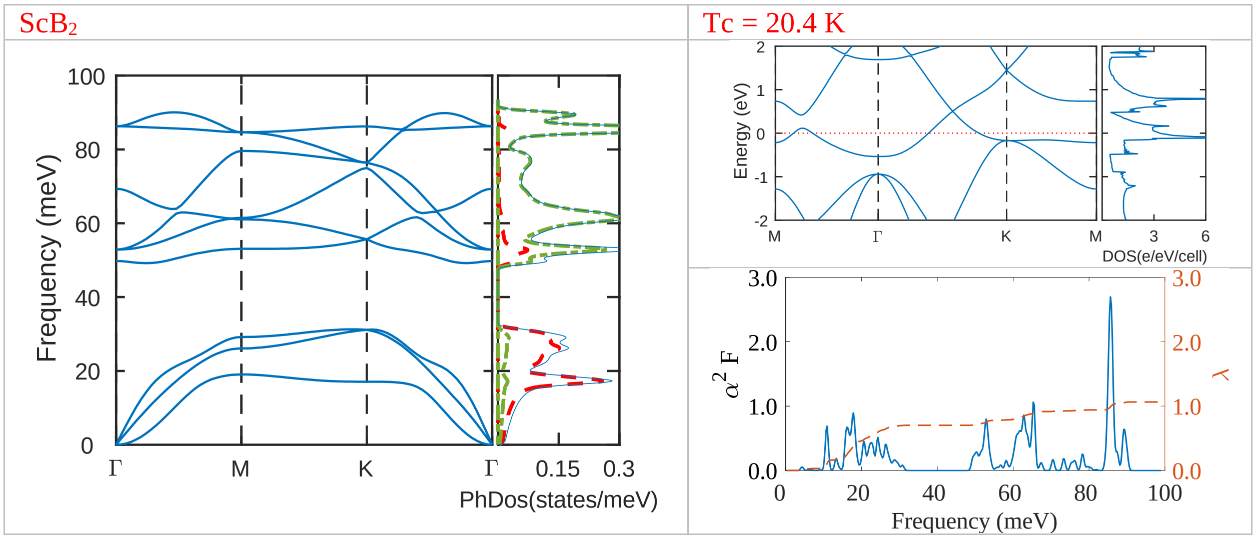
ScB₂
Tc = 20.4 K
Frequency (meV)
PhDos(states/meV)
Energy (eV)
DOS(e/eV/cell)
α² F
λ
Frequency (meV)

| $TiB_2$ | Tc = / |
|---|---|
| 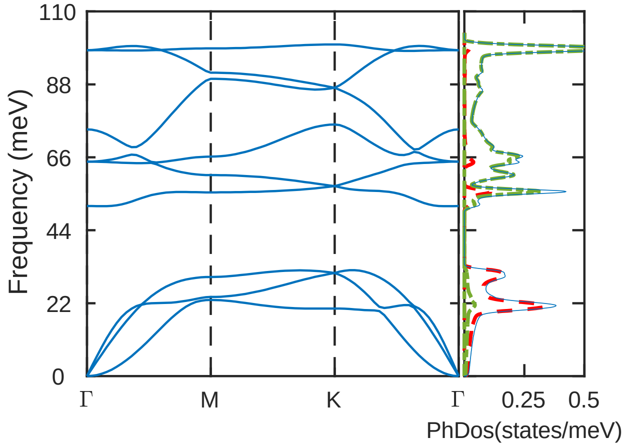 | 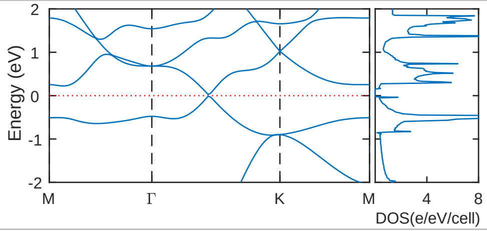 |
| | DIRAC CONE MATERIAL |



| $ZrB_2$ | Tc = 2.9 K |
|---|---|
| 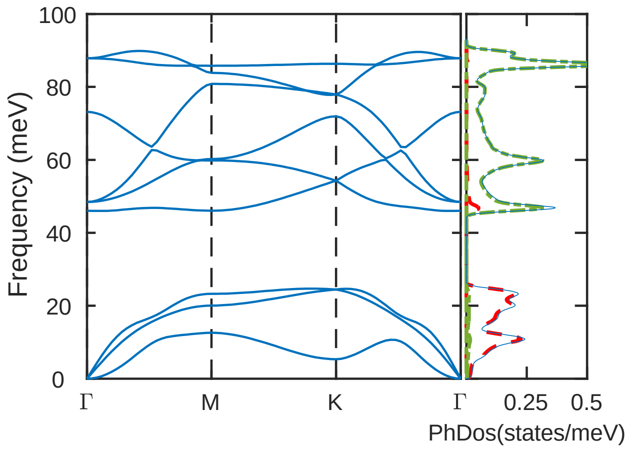 | 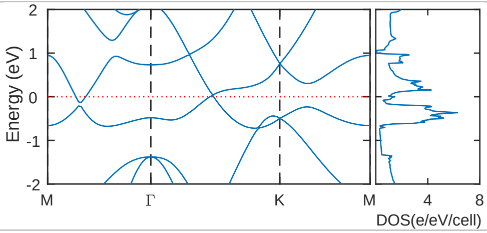 |
| | 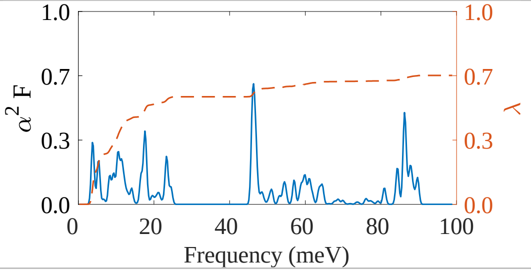 |



| $HfB_2$ | Tc = 0.8 K |
|---|---|
| 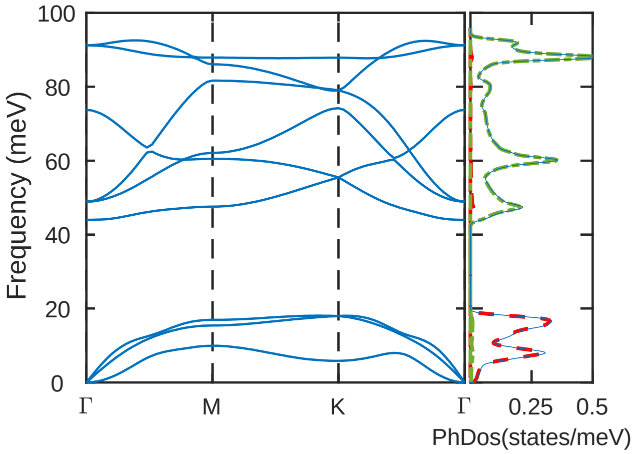 | 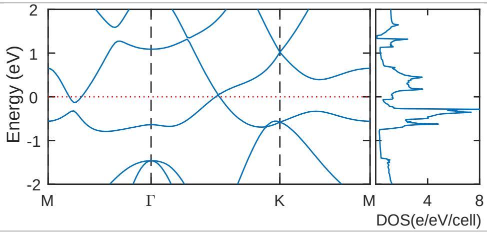 |
| | 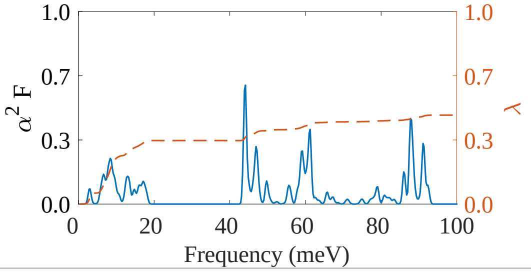 |

| $VB_2$ | Tc = 8.3 K |
|---|---|

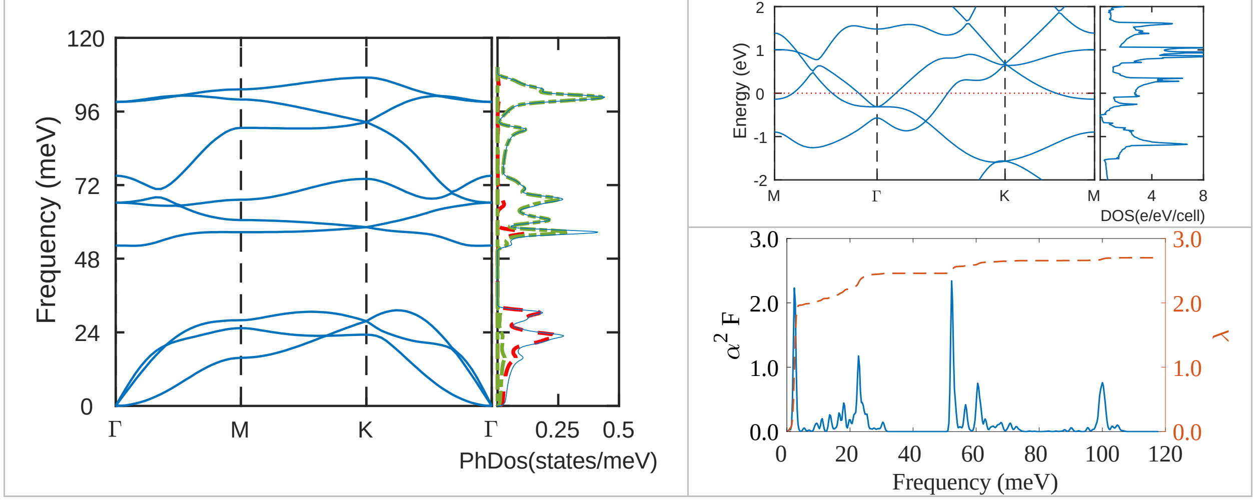


| $NbB_2$ | Tc = 35.5 K |
|---|---|

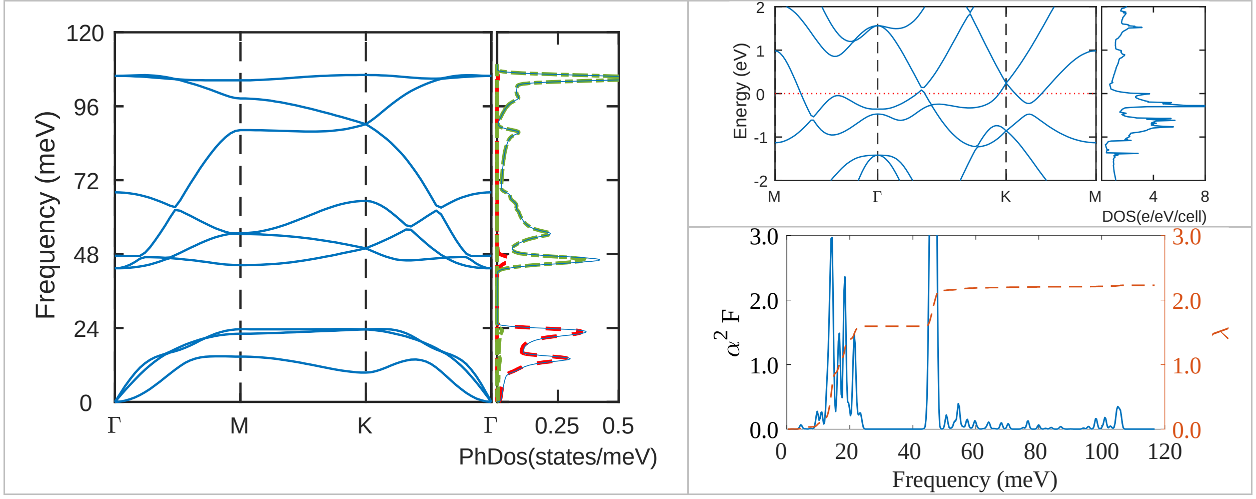


| $TaB_2$ | Tc = 7.1 K |
|---|---|

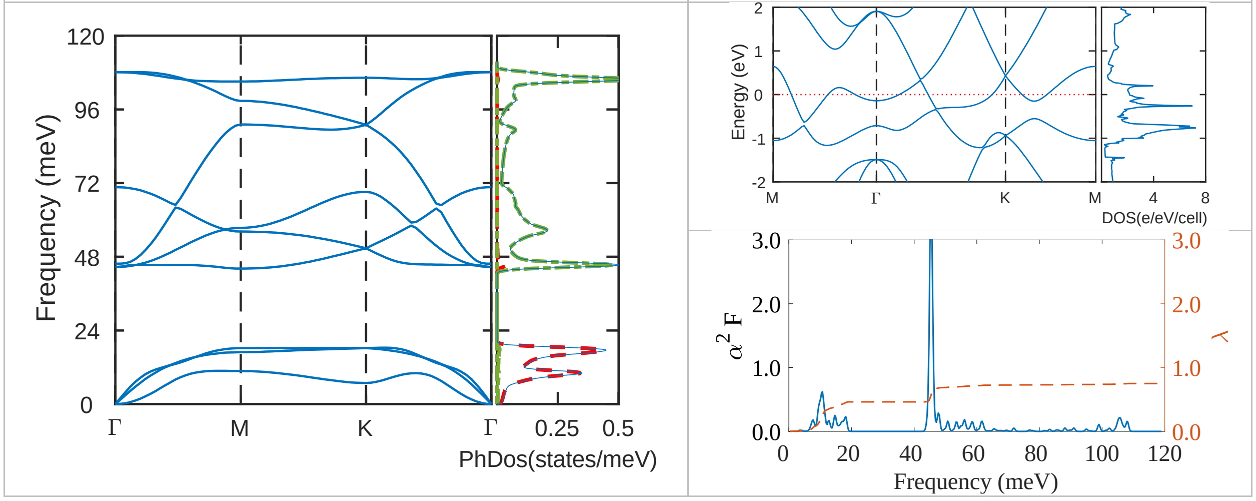

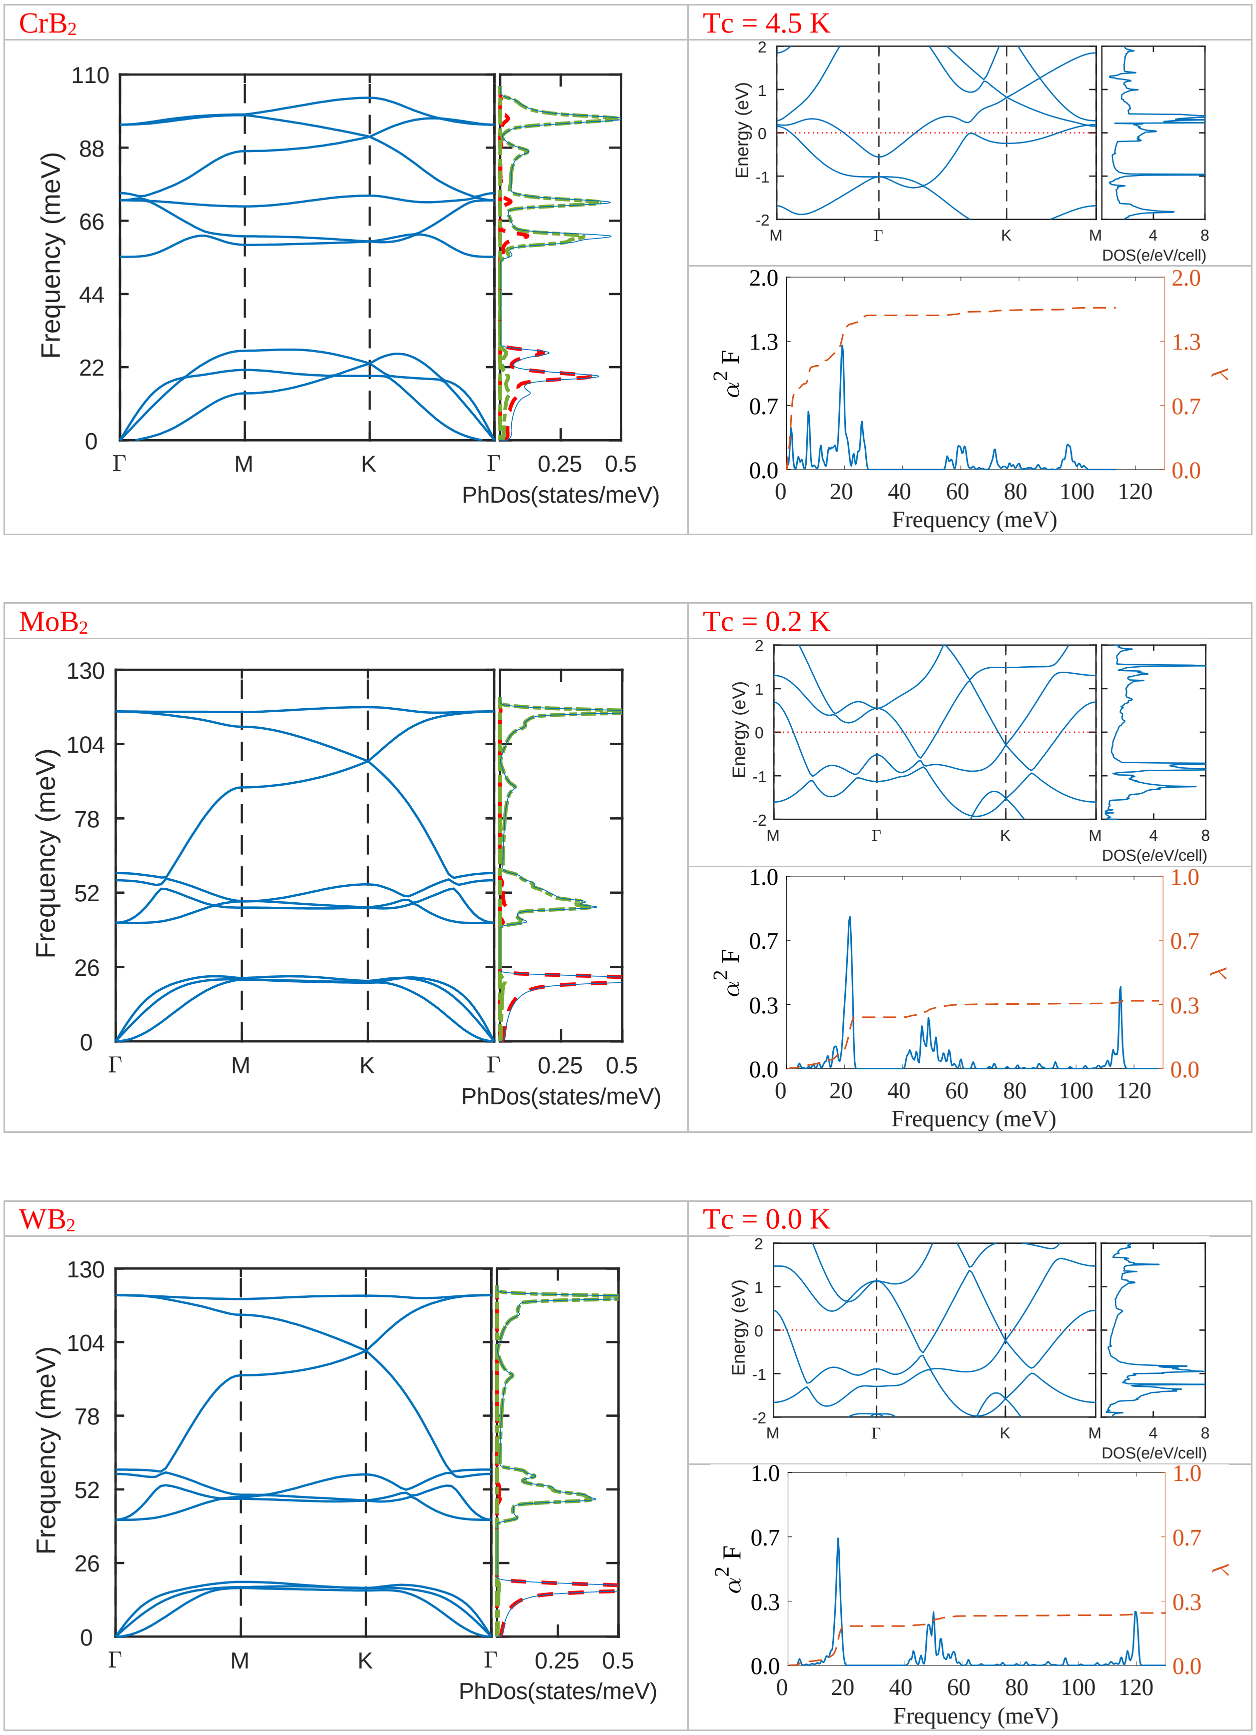

CrB2
Tc = 4.5 K
MoB2
Tc = 0.2 K
WB2
Tc = 0.0 K
Frequency (meV)
PhDos(states/meV)
Γ M K Γ
0.25 0.5
Energy (eV)
M Γ K M
DOS(e/eV/cell)
α2 F
λ
Frequency (meV)

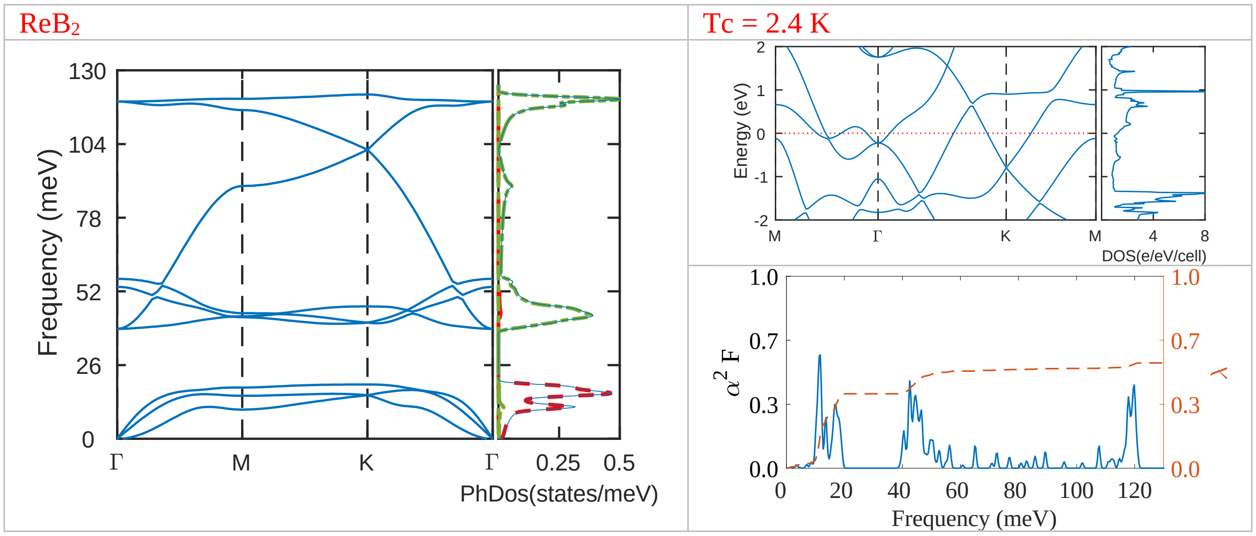

ReB2
Tc = 2.4 K
Frequency (meV)
Γ
M
K
PhDos(states/meV)
Energy (eV)
DOS(e/eV/cell)
α2 F
λ


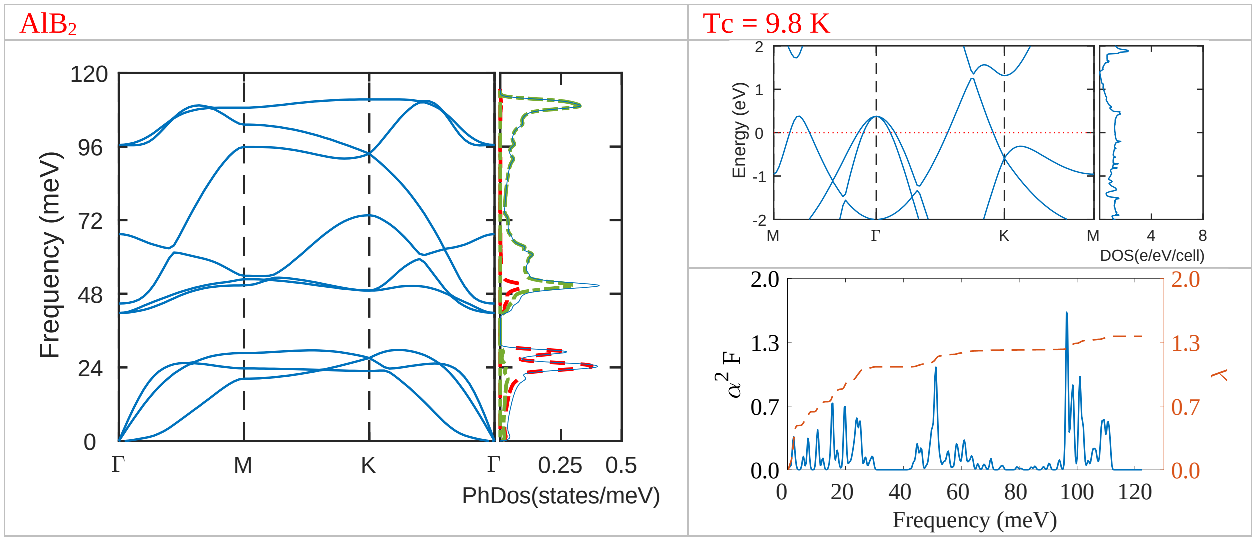

AlB2
Tc = 9.8 K
Frequency (meV)
Γ
M
K
PhDos(states/meV)
Energy (eV)
DOS(e/eV/cell)
α2 F
λ
